# Supplementary material for: Mesh Refinement for Anisotropic Diffusion in Magnetized Plasmas
Source: arXiv:2210.16442 source file (2023-06-28)
Supplement: Supplementary file 1 [file appendix-umansky.tex]

There was an attempt to verify the implementation of the discretization \eqref{eq:ssp-fem} against the semi-analytic layer width for simplified planar magnetic field problem \eqref{eq:maxim}.
\begin{figure}[htbp]
  \center
  \includegraphics[width=0.6\textwidth]{umansky_study}
  \caption{draft figure}
  \label{fig:umansky-study}
\end{figure}
The results are inconclusive at this point because of restrictions from the matlab routines that read in the MFEM solution and produce the semi-analytic routines, namely that
\begin{itemize}
  \item the routines only support serial MFEM solution... this \textit{may} be overcome by just brute forcing the serial solution
  \item the routines may only support $p=1$ output
\end{itemize}
